# Supplementary material for: Discovery of Slot Plasma Excitations in a AlGaN/GaN Plasmonic Crystal
Source: arXiv:2511.03450 source file (2025-11-05)
Supplement: Supplementary file 1 [file Supplemental_Material__2_.pdf]

# Discovery of Slot Plasma Excitations in a AlGa<sub>0.78</sub>N/GaN Plasmonic Crystal

A. R. Khisameeva<sup>a</sup>, A. Shuvaev<sup>a</sup>, I.M. Moiseenko<sup>b</sup>, P. A. Gusikhin<sup>b</sup>,  
A. S. Astrakhantseva<sup>c</sup>, A. Pimenov<sup>a</sup>, D.A. Svintsov<sup>b</sup>, I. V. Kukushkin<sup>c</sup>, V. M. Muravev<sup>c</sup> <sup>a</sup>  
<sup>a</sup> *Institute of Solid State Physics, Vienna University of Technology, 1040 Vienna, Austria*  
<sup>b</sup> *Laboratory of 2d Materials for Optoelectronics,  
Moscow Institute of Physics and Technology, Dolgoprudny, 141700 Russia*  
<sup>c</sup> *Institute of Solid State Physics, RAS, Chernogolovka, 142432 Russia*  
(Dated: November 5, 2025)

## I. DETAILED DESCRIPTION OF ALL MEASURED SAMPLES

The Al<sub>0.22</sub>Ga<sub>0.78</sub>N/GaN heterostructure used in this study were grown by molecular beam epitaxy (MBE) on semi-insulating SiC substrates. A schematic cross section of heterostructure layer composition is shown in FIG. S1(a). The two-dimensional electron gas (2DEG) layer is located beneath the surface and separated by a stack consisting of 6 nm SiN, 2 nm GaN, and 25 nm Al<sub>0.22</sub>Ga<sub>0.78</sub>N, yielding a total thickness of  $h = 34$  nm. The grating gates were formed on the sample surface by thermal evaporation of a Cr(24 nm)/Au(280 nm).

A scanning electron microscope (SEM) image of a representative plasmonic crystal grating with a period of  $p = 12$   $\mu\text{m}$ , comprising gated  $l_g = 7$   $\mu\text{m}$  and ungated  $l_u = 5$   $\mu\text{m}$  regions, is shown in FIG. S1(b).

In our study, we fabricated a series of samples with different grating-gate coupler configurations. The geometrical parameters of the structures — including the grating period, gated and ungated region lengths, filling factor, and active area — are summarized in Table I. All samples were fabricated using standard photolithography techniques.

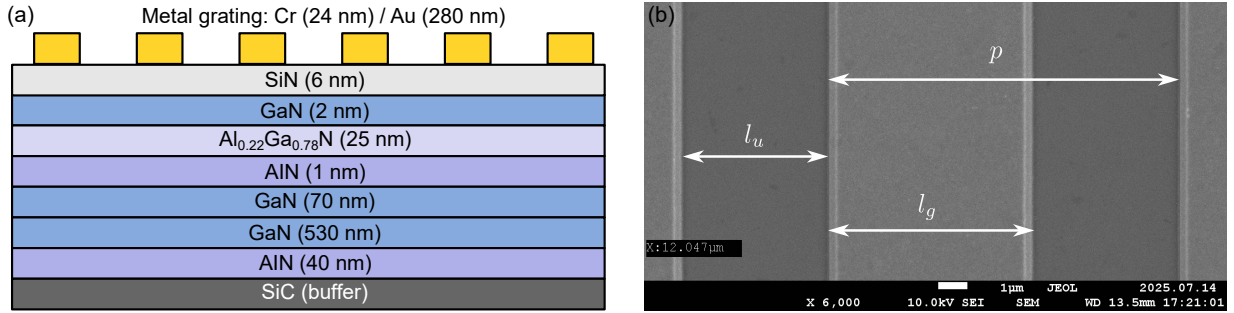

FIG. S1: (a) Schematic cross-sectional view of the plasmonic crystal structure showing the layer composition and the top metallic grating (b) SEM image of a grating segment with a period of  $p = 12$   $\mu\text{m}$ , comprising gated  $l_g = 7$   $\mu\text{m}$  and ungated  $l_u = 5$   $\mu\text{m}$  regions.

| Structure parameters                       | S1           | S2   | S3   | S4   | S5   | S6   | S7   | S8   | S9   | S10  | S11  | S12  | S13  | S14  | S15  |
|--------------------------------------------|--------------|------|------|------|------|------|------|------|------|------|------|------|------|------|------|
| Grid period $p$ , $\mu\text{m}$            | 8.0          | 8.0  | 8.0  | 8.0  | 8.0  | 8.0  | 8.0  | 8.0  | 10.0 | 12.0 | 12.0 | 16.0 | 20.0 | 24.0 | 36.0 |
| Gated region width $l_g$ , $\mu\text{m}$   | 2.8          | 3.0  | 3.1  | 4.3  | 5.0  | 5.5  | 6.2  | 6.5  | 6.1  | 7.0  | 8.6  | 8.6  | 16.6 | 12.4 | 32.3 |
| Ungated region width $l_u$ , $\mu\text{m}$ | 5.2          | 5.0  | 4.9  | 3.7  | 3.0  | 2.5  | 1.8  | 1.5  | 3.9  | 5.0  | 3.4  | 7.4  | 3.4  | 11.6 | 3.7  |
| Filling factor $f$                         | 0.35         | 0.38 | 0.39 | 0.54 | 0.63 | 0.69 | 0.77 | 0.81 | 0.61 | 0.58 | 0.72 | 0.54 | 0.83 | 0.52 | 0.90 |
| Active area, $\text{mm}^2$                 | $8 \times 8$ |      |      |      |      |      |      |      |      |      |      |      |      |      |      |

TABLE I: Parameters of the investigated plasmonic crystals.

<sup>a</sup> Corresponding E-mail: muravev@issp.ac.ru

## II. THE KRONIG-PENNEY MODEL FOR PLASMON MODES IN THE PLASMONIC CRYSTAL

In the Kronig-Penney model, the dispersion relation for a grating plasmonic crystal is derived using the following assumptions [1–5]:

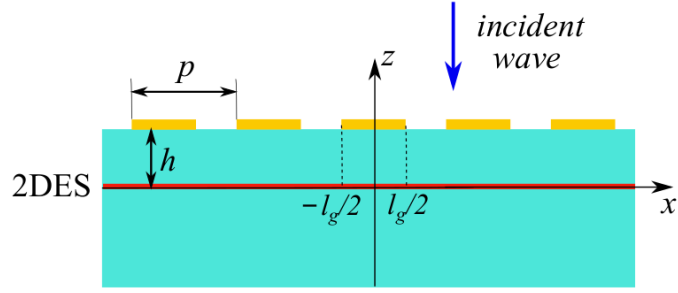

FIG. S2: Schematic of the structure under study.

1. Plane-wave expansion of the electric potential  $\varphi(x) \sim e^{iqx - i\omega t}$ . Here dispersion  $\omega(q)$  is determined by the local dispersions in each region of the 2DES.
2. Matching of the potential and electric current at the gated - ungated boundaries.
3. Imposing Bloch periodicity conditions for the fields in the adjacent gratings,  $\varphi(x + p) = \varphi(x)e^{i\Theta}$  ( $\Theta = 0$  for normal incidence).

In general, the geometry of the sample has two symmetry planes, one in the middle of the gated region and one in the middle of the ungated region, see Fig. S2. In this case, solutions can be sought in the form of symmetric and antisymmetric functions. We first consider the mode with antisymmetric potential  $\varphi$  (symmetric current density  $j$ ):

$$\begin{aligned} \varphi_g &= A_1 \sin(q_g x), & -l_g/2 < x < l_g/2 \\ \varphi_u &= A_2 \sin\left(q_u \left(x - \frac{l_g + l_u}{2}\right)\right), & p/2 > x > l_g/2 \\ \left(\varphi_u &= A_2 \sin\left(q_u \left(x + \frac{l_g + l_u}{2}\right)\right), & -p/2 < x < -l_g/2\right) \end{aligned} \quad (\text{S1})$$

The last expression for  $\varphi_u$  in the region  $x < -l_g/2$  follows from the periodic boundary condition  $\varphi(x + p) = \varphi(x)$  with  $\Theta = 0$ . Now, we relate the current density  $j$  with the potential  $\varphi$ . From the definition of the electric potential  $\mathbf{E} = -\nabla\varphi$ , and the Ohm's law  $\mathbf{j} = \sigma\mathbf{E}$ , we have:

$$j = \sigma E = -\sigma \frac{d\varphi}{dx}. \quad (\text{S2})$$

The current density for the  $j$ -symmetric mode is then:

$$\begin{aligned} j_g &= -\sigma A_1 q_g \cos(q_g x), & -l_g/2 < x < l_g/2 \\ j_u &= -\sigma A_2 q_u \cos\left(q_u \left(x - \frac{l_g + l_u}{2}\right)\right), & p/2 > x > l_g/2 \\ \left(j_u &= -\sigma A_2 q_u \cos\left(q_u \left(x + \frac{l_g + l_u}{2}\right)\right), & -p/2 < x < -l_g/2\right) \end{aligned} \quad (\text{S3})$$

We match both potential  $\varphi$  and current density  $j$  at  $x = l_g/2$  (matching at  $x = -l_g/2$  is fulfilled automatically with the choice (S1) and (S3)):

$$\begin{aligned} A_1 \sin\left(\frac{q_g l_g}{2}\right) &= -A_2 \sin\left(\frac{q_u l_u}{2}\right) \\ -\sigma A_1 q_g \cos\left(\frac{q_g l_g}{2}\right) &= -\sigma A_2 q_u \cos\left(\frac{q_u l_u}{2}\right). \end{aligned} \quad (\text{S4})$$

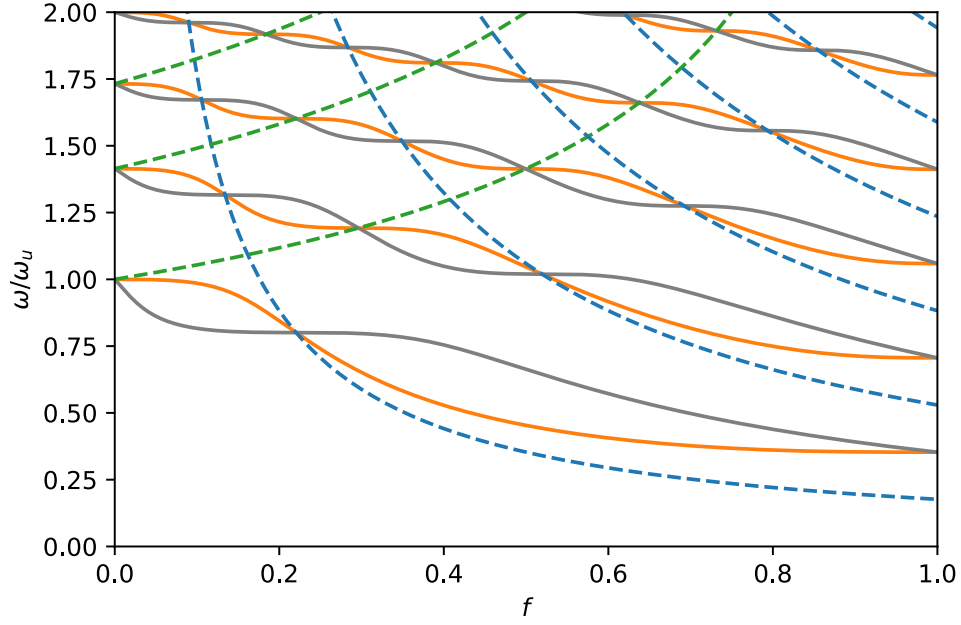

FIG. S3: Dependencies of plasmonic crystal excitation frequencies on the filling factor,  $f$ , for  $\Omega = 0.29$  (GaAs structure from the experimental work [6]). This is the **strong** coupling regime of the plasmonic crystal. Orange curves denote optically “bright” (active) plasmon modes; gray curves denote optically “dark” (inactive) modes. The dashed blue curve is the theoretical gated-plasmon dispersion from Eq. (S12) evaluated at  $q_g = M \times \pi/l_g$  ( $M = 1, 3, 5 \dots$  is an odd integer). The dashed green curve is the theoretical ungated-plasmon dispersion from the same equation evaluated at  $q_u = N \times \pi/l_u$  ( $N = 2, 4, 6 \dots$  is an even integer).

In order to have nontrivial solutions, the determinant of this system should be zero, which gives the dispersion relation for the  $j$ -symmetric mode:

$$q_u \sin\left(\frac{q_g l_g}{2}\right) \cos\left(\frac{q_u l_u}{2}\right) + q_g \cos\left(\frac{q_g l_g}{2}\right) \sin\left(\frac{q_u l_u}{2}\right) = 0. \quad (\text{S5})$$

We now determine the charge density  $\rho$  which is connected to the current density  $j$  via the continuity equation:

$$\frac{\partial \rho}{\partial t} + \text{div } \mathbf{j} = 0; \quad \frac{\partial \rho}{\partial t} + \frac{dj}{dx} = 0; \quad -i\omega\rho + \frac{dj}{dx} = 0; \quad i\omega\rho = \frac{dj}{dx}. \quad (\text{S6})$$

We have used the implied time dependency of all quantities  $\sim e^{-i\omega t}$ . The charge densities in gated and ungated regions are then:

$$\begin{aligned} i\omega\rho_g &= \sigma A_1 q_g^2 \sin(q_g x), & -l_g/2 < x < l_g/2 \\ i\omega\rho_u &= \sigma A_2 q_u^2 \sin\left(q_u \left(x - \frac{l_g + l_u}{2}\right)\right), & x > l_g/2 \\ \left(i\omega\rho_u &= \sigma A_2 q_u^2 \sin\left(q_u \left(x + \frac{l_g + l_u}{2}\right)\right), & x < -l_g/2\right) \end{aligned} \quad (\text{S7})$$

The distribution of charge density  $\rho$  is antisymmetric relative to the middle of the gated or ungated regions, implying the existence of non-zero dipole moment in both the gated and ungated zones. This means that this mode couples with the electric field of the incident radiation and can be optically excited. The symmetric distribution of the current density  $j$  is also compatible with the excitation by the homogeneous electric field of the incident radiation.

In contrast, the mode with antisymmetric current  $j$  (symmetric charge density  $\rho$ ) cannot be excited optically and can be designated as a dark mode. The derivation of the dispersion relation of the dark mode is similar. Its potential is:

$$\begin{aligned} \varphi_g &= B_1 \cos(q_g x), & -l_g/2 < x < l_g/2 \\ \varphi_u &= B_2 \cos\left(q_u \left(x - \frac{l_g + l_u}{2}\right)\right), & p/2 > x > l_g/2 \end{aligned} \quad (\text{S8})$$

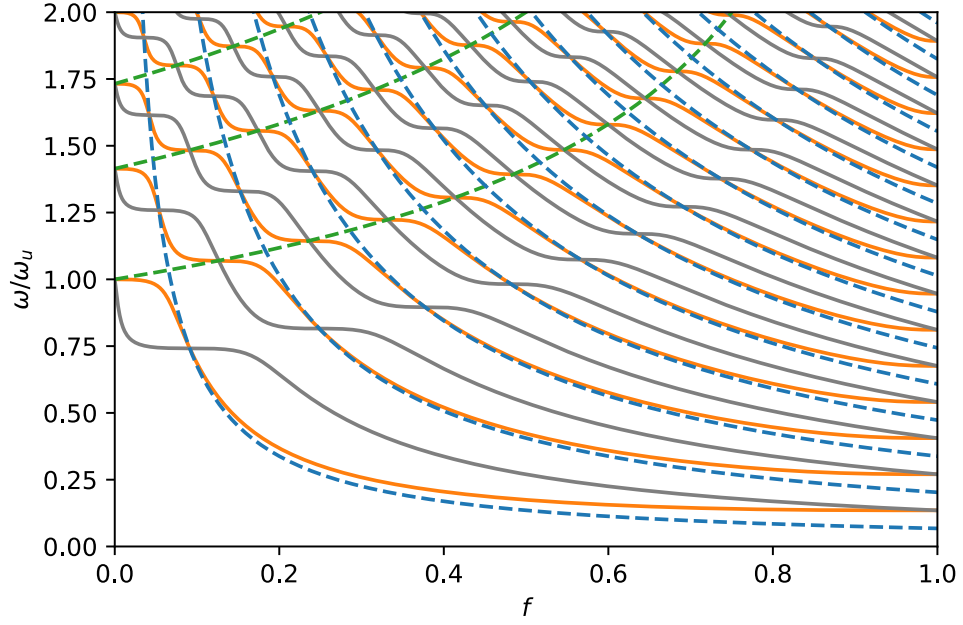

FIG. S4: Dependencies of plasmonic crystal excitation frequencies on the filling factor,  $f$ , for  $\Omega = 0.108$ . Orange curves denote optically “bright” (active) plasmon modes; gray curves denote optically “dark” (inactive) modes. The dashed blue curve is the theoretical gated-plasmon dispersion from Eq. (S12) evaluated at  $q_g = M \times \pi/l_g$  ( $M = 1, 3, 5 \dots$  is an odd integer). The dashed green curve is the theoretical ungated-plasmon dispersion from the same equation evaluated at  $q_u = N \times \pi/l_u$  ( $N = 2, 4, 6 \dots$  is an even integer).

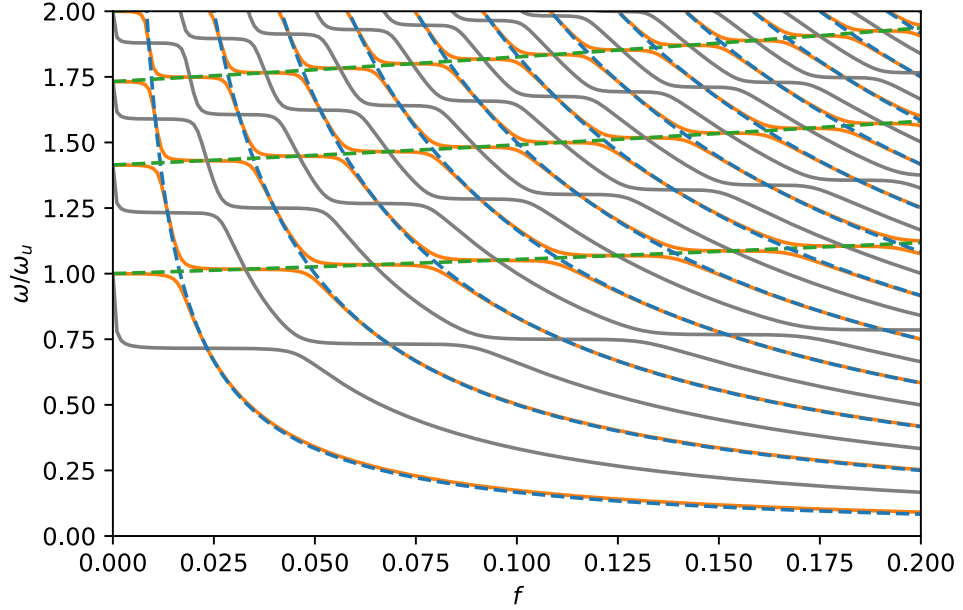

FIG. S5: Dependencies of plasmonic crystal excitation frequencies on the filling factor,  $f$ , for  $\Omega = 0.03$ . This is the **weak** coupling regime of the plasmonic crystal. Orange curves denote optically “bright” (active) plasmon modes; gray curves denote optically “dark” (inactive) modes. The dashed blue curve is the theoretical gated-plasmon dispersion from Eq. (S12) evaluated at  $q_g = M \times \pi/l_g$  ( $M = 1, 3, 5 \dots$  is an odd integer). The dashed green curve is the theoretical ungated-plasmon dispersion from the same equation evaluated at  $q_u = N \times \pi/l_u$  ( $N = 2, 4, 6 \dots$  is an even integer).

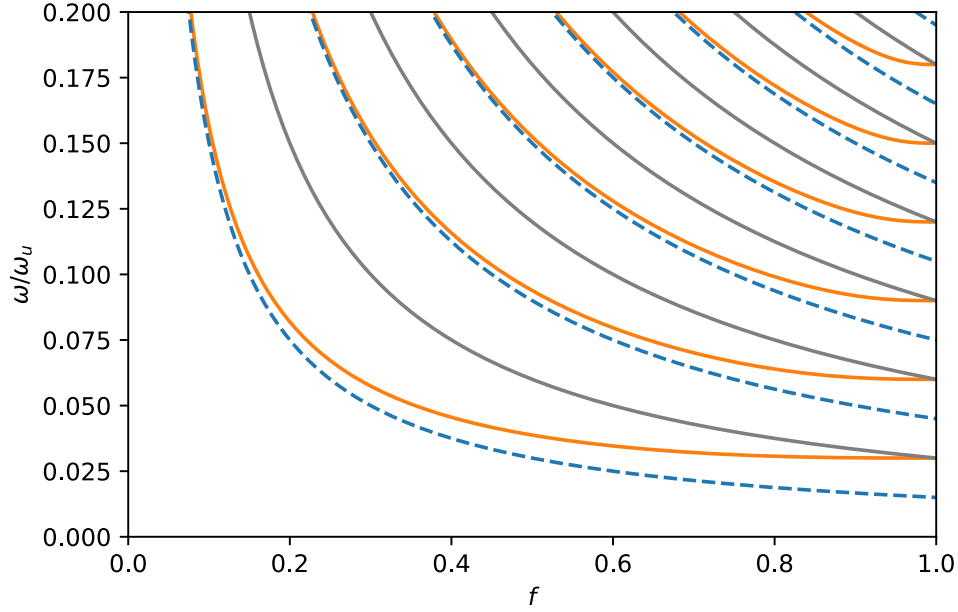

FIG. S6: Dependencies of plasmonic crystal excitation frequencies on the filling factor,  $f$ , for  $\Omega = 0.03$ . The transition between the gated plasmon with  $q_g = \pi/l_g$  and  $q_g = 2\pi/p$  is depicted.

the current density:

$$\begin{aligned} j_g &= \sigma B_1 q_g \sin(q_g x), & -l_g/2 < x < l_g/2 \\ j_u &= \sigma B_2 q_u \sin\left(q_u \left(x - \frac{l_g + l_u}{2}\right)\right), & p/2 > x > l_g/2 \end{aligned} \quad (\text{S9})$$

and the charge density:

$$\begin{aligned} i\omega\rho_g &= \sigma B_1 q_g^2 \cos(q_g x), & -l_g/2 < x < l_g/2 \\ i\omega\rho_u &= \sigma B_2 q_u^2 \cos\left(q_u \left(x - \frac{l_g + l_u}{2}\right)\right), & p/2 > x > l_g/2 \end{aligned} \quad (\text{S10})$$

The dispersion relation of the dark mode is obtained by matching potential  $\varphi$  and current density  $j$  at  $x = l_g/2$ :

$$q_u \sin\left(\frac{q_u l_u}{2}\right) \cos\left(\frac{q_g l_g}{2}\right) + q_g \sin\left(\frac{q_g l_g}{2}\right) \cos\left(\frac{q_u l_u}{2}\right) = 0. \quad (\text{S11})$$

In order to solve Eqs. (S5) and (S11) we recall that  $l_u = p - l_g$ , values of  $q_u$  and  $q_g$  are related with the frequency of the incident wave,  $\omega$ , via the dispersion equations for unscreened and screened plasmons. Namely, in the case of our system (in the limit  $\omega\tau \gg 1$  and neglecting the electromagnetic retardation effects), the relations are as follows:

$$\omega_u(q_u) = \sqrt{\frac{n_s e^2 q_u}{2m^* \varepsilon \varepsilon_0} \left(1 + \frac{\varepsilon - 1}{\varepsilon + 1} e^{-2q_u h}\right)} \quad \text{and} \quad \omega_g(q_g) = \sqrt{\frac{n_s e^2 q_g}{2m^* \varepsilon \varepsilon_0} (1 - e^{-2q_g h})}. \quad (\text{S12})$$

If the parameter  $q_{g,u} h \ll 1$ , simplified dispersion relations for gated and ungated plasmons can be used:

$$\omega_u(q_u) = \sqrt{\frac{n_s e^2 q_u}{m^* (\varepsilon + 1) \varepsilon_0}} \quad \text{and} \quad \omega_g(q_g) = \sqrt{\frac{n_s e^2 h}{m^* \varepsilon \varepsilon_0}} q_g. \quad (\text{S13})$$

Figures S3, S4, S5, and S6 show solutions of the dispersion relation (S5) by orange lines and the relation (S11) by gray lines, for structures with different parameters. We could define one parameter, which governs the picture shown in these figures. Let us use the parameter:

$$\Omega = \frac{\omega_g(2\pi/p)}{\omega_u(2\pi/p)} = \sqrt{\frac{\varepsilon + 1}{\varepsilon}} \cdot \frac{2\pi}{p} h. \quad (\text{S14})$$

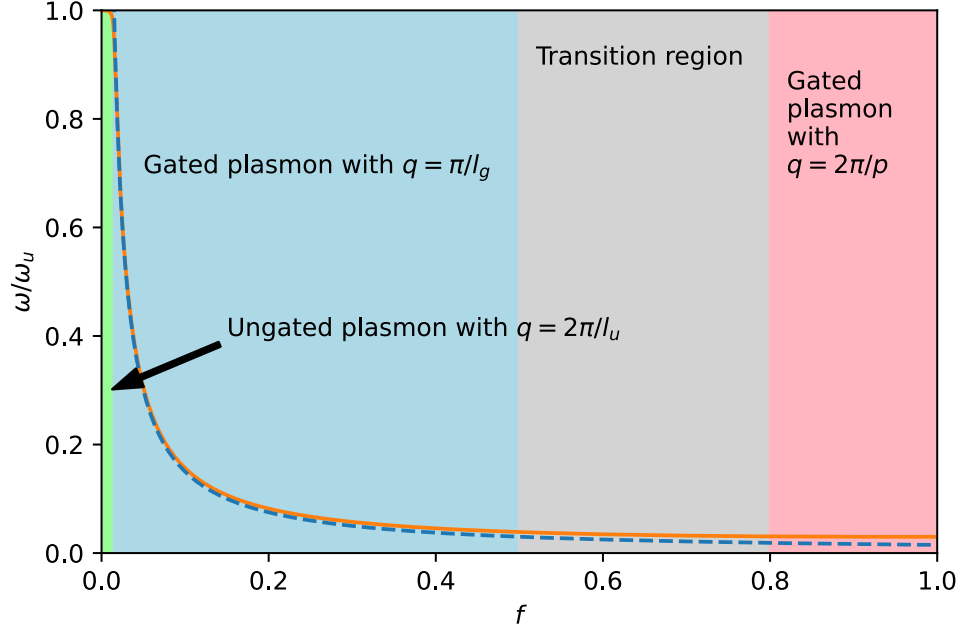

FIG. S7: Regions of the filling factor  $f$  that correspond to qualitatively different plasmonic-crystal excitation regimes: ungated plasmon with  $q_u = 2\pi/p$ , gated plasmon with  $q_g = \pi/l_g$ , transition region, and gated plasmon with  $q_g = 2\pi/p$ .

Figures S3, S4, S5, and S6 demonstrate values of the parameter  $\Omega$  equal to 0.29 (GaAs/AlGaAs structure), 0.108 (GaN/AlGaN structure), and 0.03 (hypothetical structure with extremely close gate). One can see a clear transformation of the dependencies when  $\Omega \rightarrow 0$  (or  $h/p \rightarrow 0$ ) in the figures S5 and S6. The bright mode degenerates into the set of pure single-cell modes: the ungated plasmon with wave vectors  $q = 2\pi N/l_u$  or the gated plasmon with wave vectors  $q = 2\pi(M + 1/2)/l_g$ . However, when the filling factor  $f$  becomes sufficiently large ( $f \approx 0.8$  for a fundamental mode), the frequency of the bright Kronig-Penney mode equals the frequency of the gated plasmon with the wave vector  $q = 2\pi N/p$ , the dependence on the filling factor disappears. The general dependency for the fundamental bright mode could be approximated by a simple expression:

$$\omega = \frac{\omega_g(2\pi/l_g)}{2 - f}. \quad (\text{S15})$$

Figure S7 shows the corresponding regions of the filling factor.

### III. REFLECTION OF 2D PLASMONS AT A GATE EDGE

We proceed to derive the complex reflection coefficient of 2D plasmon at the gate edge. The derivation is organized as follows. We first write down the Maxwell's equations for the 2DES covered by a semi-infinite gate and excited by an external electromagnetic wave. We simplify these equations by passing from a differential three-dimensional formulation to the integral formulation, where the field is governed by external sources and the currents in 2DES and semi-infinite gate. We exclude the 2DES currents using the Ohm's law and obtain a closed-form integro-differential equations on the currents in semi-infinite gate excited by external field. Such an approach is quite often used in numerical and semi-analytical modeling of various gated structures based on 2DES.

As the governing equation for gate currents is formulated, we are prepared for the solution of plasmon scattering problem. We 'switch off' the external sources of electromagnetic field running from infinity. Instead, we split the total electric field in the gate plane into the *known* plasmonic component (running from ungated section toward the gate edge), and scattered field component that is yet to be found. Such approach aligns with scattering problems in quantum mechanics, where the total wave function is decomposed into the incident plane wave and scattered wave, the latter having known asymptotics at infinity. The governing equation for the scattered field is Fourier transformed to the reciprocal  $q$ -space. The scattered plasmon field is found with Wiener-Hopf method. It appears to have a pole

at a complex wave vector  $-q_u$  corresponding to that of reflected plasmon. Applying the contour integration technique to pass from reciprocal  $q$ -space to the real  $x$ -space, one observes that the residue of scattered field at  $-q_u$  governs the amplitude of the reflected plasmon.

We now outline this method formally. The 2DES located at  $z = 0$  and gate at  $z = h$  are illuminated by an external plane wave with vector potential amplitude  $\mathbf{A}_{ext}$ . We retain the explicit  $z$ -dependence of all fields, and pass to the reciprocal Fourier space in the  $(x, y)$  plane, the respective wave vector is denoted by  $\mathbf{q}$ . If the currents in 2DES are denoted as  $\mathbf{j}_{2d}$  and currents in a gate – as  $\mathbf{j}_g$ , the total vector potential  $\mathbf{A}(\mathbf{q}, z)$  at any point  $z$  is given by

$$\mathbf{A}(\mathbf{q}, z) = 2\pi\mathbf{A}_{ext}\delta(\mathbf{q})e^{ik_0z} + \mathbf{j}_{2d}G(q)e^{-\kappa(\mathbf{q})|z|} + \mathbf{j}_gG(q)e^{-\kappa(\mathbf{q})|z-h|}, \quad (\text{S16})$$

where  $G(q) = 2\pi/c\kappa(q)$  is the Fourier transform of the fundamental solution of the wave equation,  $\kappa(q) = \sqrt{q^2 - k_0^2}$ . The link between vector potential and electric field in the Lorentz gauge is given by

$$\mathbf{E}_{\mathbf{q}} = \frac{i}{k_0}(k_0^2 - q^2)\mathbf{A}_{\mathbf{q}} = -\frac{i}{k_0}\kappa^2(q)\mathbf{A}_{\mathbf{q}}. \quad (\text{S17})$$

We proceed to eliminate the 2DES current by linking them to the  $\mathbf{E}$ -field with Ohm's law,  $\mathbf{j}_{2d}(\mathbf{q}) = \sigma_{2d}\mathbf{E}(\mathbf{q}, z = 0)$ . To this end, we introduce the Ohm's law in (S16), use the link between  $\mathbf{E}$  and  $\mathbf{A}$ , and write this equation once at  $z = 0$ , and second – at  $z = h$ . After some simplifications, the governing equation for the electric field in the gate plane  $z = 0$  takes the form:

$$\mathbf{E}_{\mathbf{q}}(q, z = d) = 2\pi\mathbf{E}_{ext}\delta(\mathbf{q})\frac{\varepsilon_g(q)}{\varepsilon_u(q)} - \kappa(q)\mathbf{j}_g(q)\frac{2\pi i}{ck_0}\frac{\varepsilon_g(q)}{\varepsilon_u(q)}, \quad (\text{S18})$$

where we have introduced the shorthand notations for the dielectric functions of gated ( $\varepsilon_g(q)$ ) and ungated ( $\varepsilon_u(q)$ ) 2DES:

$$\varepsilon_u(q) = 1 + \frac{2\pi i\sigma_{2d}}{c}\frac{\kappa(q)}{k_0}, \quad (\text{S19})$$

$$\varepsilon_g(q) = 1 + \frac{2\pi i\sigma_{2d}}{c}\frac{\kappa(q)}{k_0}(1 - e^{-2\kappa(q)h}). \quad (\text{S20})$$

The poles of these dielectric functions correspond to the wave vectors of the ungated and gated plasmons, which we denote at  $q = \pm q_u$  and  $q = \pm q_g$ . In the limit of weak retardation ( $|\eta| \ll 1$ ) and small gate-channel separation ( $k_0h \ll |\eta|$ ), the wave vectors are approximately given by  $q_u \approx k_0/\eta''$ ,  $q_g \approx \sqrt{k_0/(h\eta'')}$ .

We proceed to the plasmon scattering problem and set external field to zero,  $\mathbf{E}_{ext} = 0$ . From now on, we fix the polarization of the fields to the  $x$ -axis, and skip the vector notation. An ungated plasma wave is incident from the left half-space  $x < 0$  onto the gate edge occupying the complementary half-space  $x > 0$ . We choose the incident plasmon field as that bounded to  $x < 0$ , and decompose the total field as

$$E(x) = E_0e^{iq_u x}\theta(-x) + E_{scat}(x). \quad (\text{S21})$$

Performing the Fourier transform and introducing the result in (S18), we find the governing equation for the scattered field:

$$\left[ \frac{iE_0}{q - q_u} + E_{scat}(q) \right] M(q) + \frac{i}{2}j_g Z_0 = 0, \quad (\text{S22})$$

$$M(q) = \frac{\varepsilon_u(q)k_0}{\varepsilon_g(q)\kappa(q)}, \quad (\text{S23})$$

here we have introduced the free-space impedance  $Z_0 = 4\pi/c$ . Now we are ready to apply the Wiener Hopf method to the equation (S22) governing the scattered field. It is based on splitting all emerging functions into those analytic in the upper (UHP) and lower (LHP) half planes of the complex wave vector variable  $q = q' + iq''$ . The gate current  $j_g(x)$  is bounded to  $x > 0$ , therefore its Fourier transform  $j_g(q)$  is analytic in the LHP. The electric field  $E_{scat}(x)$  does not penetrate into the gate and is bounded to  $x < 0$ , therefore  $E_{scat}(q)$  is analytic in the UHP. All other functions entering (S22) are decomposed as products of UHP-analytic functions, which we supplement with index  $+$ , and LHP analytic functions, which we supplement with index  $-$ . In particular,  $M(q) = M_+(q)M_-(q)$ . The multiplicative decomposition for an arbitrary function  $M(q)$  can be reached with Cauchy theorem

$$M_{\pm}(q) = \exp \left\{ \pm \frac{1}{2\pi i} \int_{-\infty}^{+\infty} \frac{\ln M(u) du}{u - (q \pm i\delta)} \right\}. \quad (\text{S24})$$

After all functions are decomposed into UHP-analytic and LHP-analytic, and the governing equation (S18) is presented as  $f_+(q) = g_-(q)$ , we are ready to state that both  $f_+(q)$  and  $g_-(q)$  are identically zero. More precisely, both functions are equal to an entire function in the whole complex  $q$ -plane, which can be only a polynomial. Still, if this polynomial is non-zero, the inverse Fourier transforms of the fields would become divergent, thus zero function is an only remaining option.

After the decomposition, the solution for the scattered field appears as

$$E_{\text{scat}}(q) = -\frac{iE_0}{q - q_u} \left[ 1 - \frac{M_+(q_u)}{M_+(q)} \right]. \quad (\text{S25})$$

The solution has a pole at  $q = -q_u$ , which is reached with the following observation. Expression (S25) contains  $\varepsilon_{u+}(q)$  in the denominator. By multiplicative decomposition,  $\varepsilon_{u+}(q) = \varepsilon_u(q)/\varepsilon_{u-}(q)$ , where  $\varepsilon_u(q)$  has zeros at  $q = \pm q_u$ , and  $\varepsilon_{u-}(q)$  is free of poles and zeros in the LHP, which retains the zero at  $q = -q_u$  uncompensated. Evaluation of the residue of the scattered field at  $q = -q_u$  yields the amplitude of the reflected plasma wave:

$$E_r \equiv rE_0 = \text{Res}_{q=-q_u} \frac{E_0}{q - q_u} \frac{M_+(q_u)}{M_+(q)} \quad (\text{S26})$$

The residue is evaluated as

$$r = -\frac{i}{2q_u} \left[ \frac{\varepsilon_{u+}(q_u)}{\varepsilon_{g+}(q_u)} \right]^2 \sqrt{\frac{q_u/k_0 - 1}{q_u/k_0 + 1}} \frac{e^{-2\kappa(q_u)h}}{\partial \varepsilon_u / \partial q|_{q=-q_u}}. \quad (\text{S27})$$

Considerable simplifications of this expression are possible in weakly dissipative ( $\eta' \ll \eta''$ ) non-retarded ( $|\eta| \ll 1$ ) limit. The reflection coefficient becomes

$$r = -i \exp(i\pi/4 - i\phi_g) \left[ \frac{1 - q_u/q_g}{1 + q_u/q_g} \right], \quad (\text{S28})$$

where the phase of the gated dielectric split function  $\phi_g$  is given by

$$\phi_g = -\frac{1}{\pi} \int_{-\infty}^{+\infty} \ln \left| \frac{\varepsilon_g(u)}{1 - u^2/q_u^2} \right| \frac{du}{u + q_u}. \quad (\text{S29})$$

The latter phase approaches zero in the limit of proximate gates  $q_u h \ll 1$ , and acquires a linear correction  $O(q_u h)$  at small  $h$ .

In the limit of small gate-channel separation, the total phase acquired by reflected plasmon equals  $7\pi/4$ , of which  $\pi$  as the normal phase shift expected for reflection from opaque objects,  $\pi/2$  as the additional phase shift provided by the sharp metal edge of the gate, and  $\pi/4$  as the nontrivial shift arising from the excitation of evanescent fields at the edges of the unscreened 2DES. The obtained result contrasts with plasmon reflection from the terminated edge of the 2DES, where the phase shift is  $\pi + \pi/4 = 5\pi/4$ . The physical origin of the  $\pi/2$  phase difference between the considered two cases is the presence of strong electric fields near the metallic gate edge.

#### IV. MAGNETIC-FIELD MEASUREMENT RESULTS

The magnetic-field measurements were performed in the Faraday geometry, with the magnetic field applied perpendicular to the sample plane, using an optical cryostat equipped with a split-coil superconducting magnet capable of fields up to 7 T. The setup was integrated with a fiber-based THz time-domain spectroscopy (THz-TDS) system. All data were acquired at a base sample temperature of  $T = 1.8$  K.

Figure S8(a) shows the THz-TDS transmission spectra of the plasmonic crystal with period  $p = 10$   $\mu\text{m}$  and filling factor  $f = 0.61$  under an applied magnetic field  $B$ . The blue and red arrows mark the cyclotron resonance and the slot-plasmon resonance, respectively. Measurements were taken for  $B = 0 - 7$  T in 1 T increments. The magnetodispersion, plotted in Fig. S8(b), exhibits a clear hybridization between the slot-plasmon mode (red symbols) and the cyclotron resonance (blue symbols). The resulting upper hybrid mode follows

$$\omega^2 = \omega_u^2 + \omega_c^2 \quad (\text{S30})$$

where the cyclotron frequency is  $\omega_c = eB/m^*$  and  $\omega_u$  is the zero-field frequency of the slot plasmon. The experimental data closely follow the theoretical fit. From the field dependence of the cyclotron resonance, we extract an effective electron mass of  $m^* = 0.24 m_0$ , which is used in the subsequent analysis.

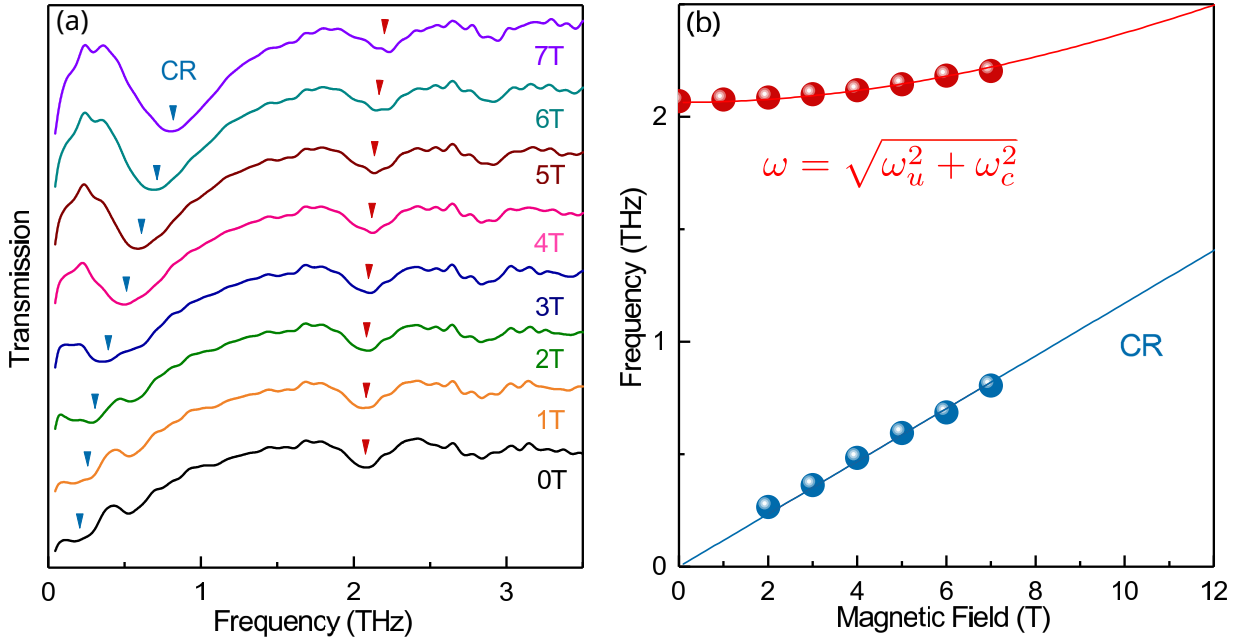

FIG. S8: (a) Transmission spectra of the plasmonic crystal with period  $p = 10$   $\mu\text{m}$  and filling factor  $f = 0.61$  under applied magnetic field. Blue arrows mark the cyclotron resonance (CR); red arrows indicate the slot-plasmon mode. (b) Magnetodispersion of both modes. The blue line shows the cyclotron frequency  $\omega_c = eB/m^*$ , and the red line shows the dispersion given by Eq. (S30). Blue and red dots are experimental data for the CR and slot-plasmon mode, respectively.

## V. DETAILED TEMPERATURE-DEPENDENT MEASUREMENTS

Figure S9 shows the temperature evolution of the THz transmission spectra for plasmonic crystals with identical slot widths,  $l_u = 4.0 \mu\text{m}$ , but different gated regions: (a)  $l_g = 6 \mu\text{m}$  and (b)  $l_g = 8 \mu\text{m}$ . Notably, the plasmon resonance remains clearly observable under ambient conditions. The slot-plasmon mode is essentially unchanged up to  $T = 125 \text{ K}$ , after which its amplitude gradually decreases. The extracted temperature dependence of the linewidth for both samples, presented in Fig. S9(c).

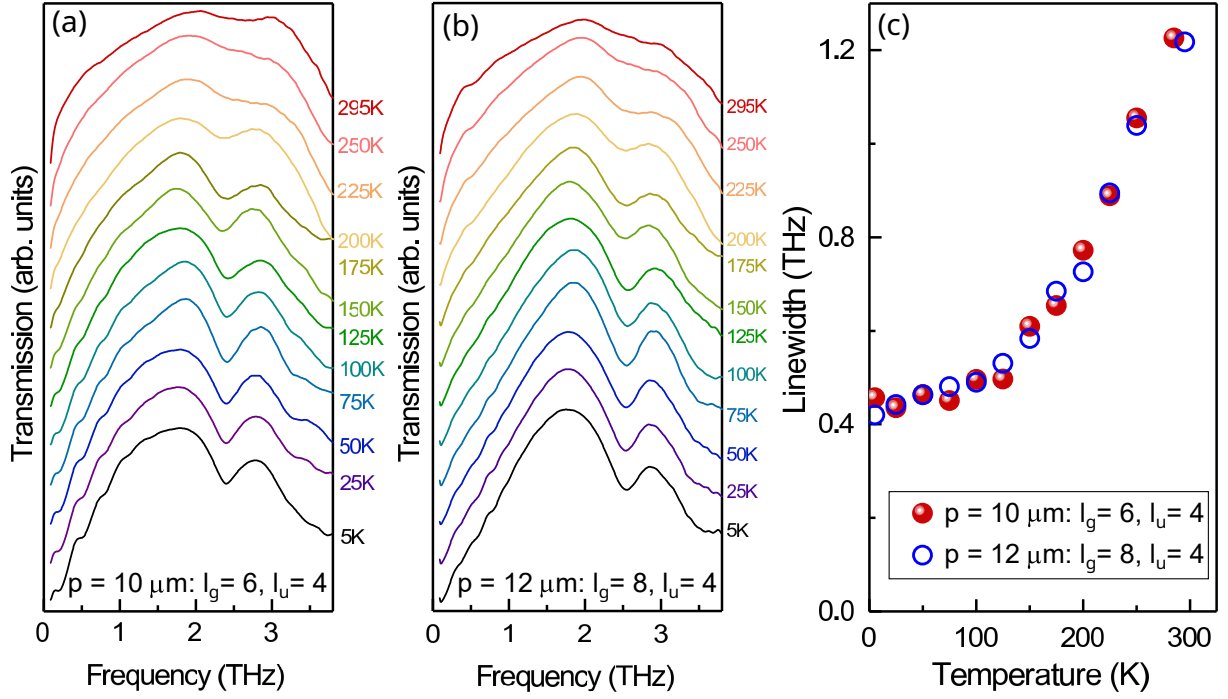

FIG. S9: Temperature-dependent THz transmission spectra from 5 to 300 K for plasmonic crystals with (a)  $l_u = 4 \mu\text{m}$  and  $l_g = 6 \mu\text{m}$ , (b)  $l_u = 4 \mu\text{m}$  and  $l_g = 8 \mu\text{m}$ . (c) Extracted linewidth of the slot-plasmon mode versus temperature for both samples.

- 
- [1] G. R. Aizin and G. C. Dyer, Transmission line theory of collective plasma excitations in periodic two-dimensional electron systems: Finite plasmonic crystals and Tamm states, *Phys. Rev. B* **86**, 235316 (2012).
  - [2] V. V. Popov, D. V. Fateev, E. L. Ivchenko, and S. D. Ganichev, Noncentrosymmetric plasmon modes and giant terahertz photocurrent in a two-dimensional plasmonic crystal, *Phys. Rev. B* **91**, 235436 (2015).
  - [3] V. Y. Kachorovskii and M. S. Shur, Current-induced terahertz oscillations in plasmonic crystal, *Appl. Phys. Lett.* **100**, 232108 (2012).
  - [4] A. Bylinkin, E. Titova, V. Mikheev, E. Zhukova, S. Zhukov, M. Belyanchikov, M. Kashchenko, A. Miakonkikh, and D. Svin'tsov, Tight-binding terahertz plasmons in chemical-vapor-deposited graphene, *Phys. Rev. Applied* **11**, 054017 (2019).
  - [5] I. Gorbenko and V. Kachorovskii, Lateral plasmonic crystals: Tunability, dark modes, and weak-to-strong coupling transition, *Phys. Rev. B* **110**, 155406 (2024).
  - [6] A. R. Khisameeva, A. Shuvaev, A. A. Zabolotnykh, A. S. Astrakhantseva, D. A. Khudaiberdiev, A. Pimenov, I. V. Kukushkin, and V. M. Muravev, Spectrum of plasma excitations in a plasmonic crystal fabricated in an algaas/gaas heterostructure, *Phys. Rev. Res.* **7**, 033224 (2025).
